# Supplementary material for: Sharp symbolic nonparametric bounds for measures of benefit in observational and imperfect randomized studies with ordinal outcomes
Source: arXiv:2305.10555 ancillary file (2023-05-17)
Supplement: Supplementary file 1 [file supplement.pdf]

# Supplementary Materials: Sharp symbolic nonparametric bounds for measures of benefit in observational and imperfect randomized studies with ordinal outcomes

## Table of contents


**Notation** 1

**Proofs** 2

**Noncompliance No Assumptions** 5

Bounds for $\phi$ . . . 5

Number of levels of $Y$: 3 . . . 5

**Noncompliance with no defiers** 8

Bounds for $\psi$ . . . 8

Number of levels of $Y$: 4 . . . 8

Number of levels of $Y$: 5 . . . 8

Bounds for $\theta$ . . . 9

Number of levels of $Y$: 4 . . . 9

Number of levels of $Y$: 5 . . . 9

Bounds for $\phi$ . . . 10

Number of levels of $Y$: 4 . . . 10

Number of levels of $Y$: 5 . . . 10


## Notation

$$p_{xy\cdot z} = P(X = x, Y = y|Z = z)$$

$$p_{xy} = P(X = x, Y = y)$$

By Theorem 1 of Sachs et al. [2022], in the confounded setting, there exists a canonical partitioning of the unmeasured confounder $U$ into a pair of categorical response function variables $R_x$ (two levels) and $R_y$ ($K^2$ levels) such that for any $u$ in the range of $U$ and $x \in \{0, 1\}$, there exists an $r_x, r_y$ and response function $f_Y$ such that $g_Y(u, x) = f_Y(r_y, x)$. For $X$, which has no parents other than $U$, there is also a function $f_X$ and value $r_x$ such that $g_X(u) = f_X(r_x)$ for any $u$. The joint distribution of $(R_x, R_y)$, called the response function variables, together with the response functions $f_Y, f_X$ fully characterize the causal model.

Let $q_{R_xR_y}$ be the response function variable probabilities that define the possible responses of $Y$, given $X$, and potentially the ancestors of $X$, $U$ and any random independent errors. For example, $q_{1m}$, is the probability of one possible response pattern of $Y$ when $X = 1$. Thus the observed joint probabilities can be written as all possible response functional counterfactual probabilities which lead to the observed values in the joint.

# Proofs

**Proof Theorem 1**:
Theorem 1: In the setting of DAG b in Figure 1, the tight and valid bounds for $\psi = P\{Y_i(1) \geq Y_i(0)\}$, for a discrete $Y$ with arbitrary levels $K$ is given by:

$$p_{00} + p_{1(K-1)} \leq \psi \leq 1.$$

Proof: First the observable joint probabilities can be written in terms of the $q$ as:

$$p_{00} = \sum_{\{R_x, R_y : X=0, Y=0\}} q_{R_xR_y}$$

$$p_{1(K-1)} = \sum_{\{R_x, R_y : X=1, Y=K-1\}} q_{R_xR_y}$$

and

$$\begin{aligned} \psi &= p\{Y(1) = 0, Y(0) = 0\} + p\{Y(1) = 1, Y(0) \leq 1\} + \\ &\quad p\{Y(1) = 2, Y(0) \leq 2\} + \ldots + p\{Y(1) = K-1, Y(0) \leq K-1\} \\ &= \sum_{\{R_x, R_y : f_Y(x=1, R_y) \geq f_Y(x=0, R_y)\}} q_{R_xR_y} \end{aligned}$$

Since $X$ has no parents in the confounded setting other than the confounder $U$, the set

$$\{R_x, R_y : f_Y(x=1, R_y) \geq f_Y(x=0, R_y)\}$$

contains $\{R_x, R_y : X = 0, Y = 0\}$ and $\{R_x, R_y : X = 1, Y = K-1\}$ because the observations $X = 0, Y = 0$ and $X = 1, Y = K-1$ can only be the result of a response function in which $f_Y(x = 1) \geq f_Y(x = 0)$. Since $Y$ cannot be less than 0 and cannot exceed $K - 1$, then

$$\psi = \sum_{\{R_x,R_y:X=0,Y=0\}} q_{R_xR_y} + \sum_{\{R_x,R_y:X=1,Y=K-1\}} q_{R_xR_y} + Q$$

where $Q$ is some the sum of response functional counterfactual probabilities in $\psi$, but not in $p_{00}$ of $p_{1(K-1)}$. Thus, $p_{00} + p_{1(K-1)} \leq \psi$, and, as $\psi$ is always $\leq 1$ as it is a probability, we have now proven that $p_{00} + p_{1(K-1)} \leq \psi \leq 1.$, are valid bounds for $\psi$.

To show they are tight, we look at Q, which are all parts of $\psi$ not contained in either $p_{00}$ or $p_{1K-1}$ $Q = p\{Y(1) = 1, Y(0) = 1\}+p\{Y(1) = 2, 0 < Y(0) \leq 2\} \ldots p\{Y(1) = K-2, 0 < Y(0) \leq K-2\}$, There is no $p_{xy}$ that is contained completely in this set, which $p_{01}$, having the largest overlap, only lacking $p\{Y(1) = 0, Y(0) = 1\}$ and $p\{Y(1) = K-1, Y(0) = 1\}$, with $p\{Y(1) = 0, Y(0) = 1\}$ not being represented in the objective even within $p_{00} + p_{1(K-1)}$. Thus, we cannot add more $p_{xy}$ to the lower bound without risking making the bounds invalid without further assumptions. Thus, the lower bound is tight. Additionally, adding any constant is impossible without further assumptions or restrictions, as all parts of $Q$ can equal zero.

$Q$ contains at least one $q_{R_xR_y}$ for each of the observable $p_{xy}$, other than $p_{00} + p_{1(K-1)}$. Thus any upper bound must contain $p_{00} + p_{1(K-1)}$, and all other observed joints, and therefore 1 is a tight bound, as additional information would be needed to remove any observable joint.

**Proof Theorem 2**:
Theorem 2: In the setting of DAG b in Figure 1 the tight and valid bounds for $\theta = P\{Y_i(1) > Y_i(0)\}$, for a discrete $Y$ with arbitrary levels $K$ is given by:

$$0 \leq \theta \leq 1 - p_{10} - p_{0(K-1)}.$$

$$p_{10} = \sum_{\{R_x,R_y:X=1,Y=0\}} q_{R_xR_y}$$

$$p_{0(K-1)} = \sum_{\{R_x,R_y:X=0,Y=K-1\}} q_{R_xR_y}$$

Proof:

$$\begin{aligned}\theta &= p\{Y(1) = 1, Y(0) = 0\} + p\{Y(1) = 2, Y(0) < 2\} + \ldots + p\{Y(1) = K-1, Y(0) < K-1\} \\ &= \sum_{\{R_x,R_y:f_Y(x=1,R_y)>f_Y(x=0,R_y)\}} q_{R_xR_y}\end{aligned}$$

Similar to the argument in the proof of theorem 1 for the upper bound, the objective does not contain any of the observable joint probabilities completely. Thus, the lower bound of zero cannot be improved upon without further constraints that set one or more of the response functional counterfactual probabilities to zero. As the objective is a probability, it can never be less than zero. Thus, the lower bound of zero is both valid and tight.

The two observable joints $p_{10}$ and $p_{0(K-1)}$ have no response functional probabilities in common with the objective, as $Y(1)$ must be greater than zero to be strictly greater than any value of $Y(0)$, and any response function in $p_{0(K-1)}$ would result in a $Y(0)$ that is at minimum equal to $Y(1)$. All other observable joint probabilities have at least one common response functional counterfactual probabilities with the objective. Thus, they must be included in the upper bound, for it to be valid. This is also why we cannot improve the upper bound without additional information about constraints that set the response functional counterfactual probabilities in the objective to zero. Thus, the upper bounds are both valid and tight.

**Proof Theorem 3**:
Theorem 3: In the setting of DAG b in Figure 1, the tight and valid bounds for $\phi = p\{Y_i(1) > Y_i(0)\} - p\{Y_i(1) < Y_i(0)\}$, for a discrete $Y$ with arbitrary levels $k$, is given by:

$$p_{00} + p_{1(K-1)} - 1 \leq \phi \leq 1 - p_{10} - p_{0(K-1)}.$$

$$\begin{aligned}
\phi &= [p\{Y(1) = 1, Y(0) = 0\} + p\{Y(1) = 2, Y(0) < 2\} + \ldots + p\{Y(1) = K-1, Y(0) < K-1\}] \\
&- [p\{Y(1) = 0, Y(0) = 1\} + p\{Y(1) < 2, Y(0) = 2\} + \ldots + p\{Y(1) < K-1, Y(0) = K-\}] \\
&= [p\{Y(1) = 1, Y(0) = 0\} + p\{Y(1) = 2, Y(0) < 2\} + \ldots + p\{Y(1) = K-1, Y(0) < K-1\}] \\
&- [1 - \{p\{Y(1) = 1, Y(0) = 0\} + p\{Y(1) = 2, Y(0) < 2\} + \ldots + p\{Y(1) = K-1, Y(0) < K-1\}] \\
&- [p\{Y(1) = 0, Y(0) = 0\} + p\{Y(1) = 2, Y(0) = 2\} + \ldots + p\{Y(1) = K-1, Y(0) = K-1\}] \\
&= 2[p\{Y(1) = 1, Y(0) = 0) + p\{Y(1) = 2, Y(0) < 2\} + \ldots + p\{Y(1) = K-1, Y(0) < K-1\}] \\
&+ [p\{Y(1) = 0, Y(0) = 0) + p\{Y(1) = 2, Y(0) = 2\} + \ldots + p\{Y(1) = K-1, Y(0) = K-1] - 1 \\
&= \psi + \theta - 1 \\
&= \sum_{\{R_x, R_y : f_Y(x=1, R_y) \geq f_Y(x=0, R_y)\}} q_{R_x R_y} + \sum_{\{R_x, R_y : f_Y(x=1, R_y) > f_Y(x=0, R_y)\}} q_{R_x R_y} - 1
\end{aligned}$$

As highlighted above in the proofs for $\psi$ and $\theta$, $p_{00}$ and $p_{1K-1}$ are the only observable joint probabilities fully contained in response functional probabilities within $\psi$ and $\theta$. Thus, we can include them and still have valid bounds. Additionally, as above, they are the only observable joints that can be included and removed from one without additional assumptions. Similarly, no fixed constant can be removed or added. Thus, the lower bound is tight.

The upper bound must contain 1, as all joint observable probabilities share at least one response functional probability with $\psi$. Similarly, $p_{10}$ and $p_{0K-1}$ are the only joint observable with no common response functional probabilities with $\theta$. This results in a valid upper bound for $\psi + \theta$

of $2 - p_{10} - p_{0K-1}$, and of $1 - p_{10} - p_{0K-1}$ subtracting the additional -1 in $\phi$. This bound is valid. It is also tight, as further assumptions would be needed to subtract any additional joint observable probabilities for 1, and for the bounds to remain valid, using the same reasoning as above in the proofs for $\psi$ and $\theta$.

## Noncompliance No Assumptions

### Bounds for $\phi$

#### Number of levels of $Y$: 3

**Result S1**:
In the setting of DAG c in Figure 1, the tight and valid bounds for $\phi = p(Y_i(1) > Y_i(0)) - p(Y_i(1) < Y_i(0))$, for a discrete $Y$ with three levels $\{0, 1, 2\}$ is given by:

$$
\begin{aligned}
\phi \geq \max\{ & -p_{00\cdot0} - 2p_{10\cdot0} - 2p_{01\cdot0} - p_{11\cdot0} - 2p_{02\cdot0} + p_{00\cdot1} + p_{10\cdot1} + p_{01\cdot1}, \\
& -p_{00\cdot0} - 2p_{10\cdot0} - 2p_{01\cdot0} - 3p_{11\cdot0} - 3p_{02\cdot0} + p_{00\cdot1} + p_{10\cdot1} + p_{01\cdot1} + 2p_{11\cdot1}, \\
& -p_{00\cdot0} - 2p_{10\cdot0} - 2p_{01\cdot0} - 2p_{11\cdot0} - 2p_{02\cdot0} + p_{00\cdot1} + p_{10\cdot1} + p_{01\cdot1} + p_{11\cdot1}, \\
& -p_{00\cdot0} - 2p_{10\cdot0} - 2p_{01\cdot0} - p_{11\cdot0} - p_{02\cdot0} + p_{00\cdot1} + p_{01\cdot1}, \\
& -2p_{10\cdot0} - 2p_{01\cdot0} - p_{11\cdot0} - p_{02\cdot0} + p_{01\cdot1}, \\
& p_{00\cdot0} - 2p_{10\cdot0} - 2p_{01\cdot0} - p_{11\cdot0} - p_{02\cdot0} - p_{00\cdot1} - p_{10\cdot1} + p_{01\cdot1}, \\
& -p_{00\cdot0} - 2p_{10\cdot0} - 2p_{01\cdot0} - p_{11\cdot0} + p_{00\cdot1} - p_{10\cdot1} + p_{01\cdot1} - p_{11\cdot1} - p_{02\cdot1}, \\
& p_{00\cdot0} - 2p_{10\cdot0} - 2p_{01\cdot0} - p_{11\cdot0} - p_{00\cdot1} - p_{10\cdot1} + p_{01\cdot1} - p_{11\cdot1} - p_{02\cdot1}, \\
& p_{01\cdot0} - 2p_{10\cdot1} - 2p_{01\cdot1} - p_{11\cdot1} - p_{02\cdot1}, \\
& p_{00\cdot0} + p_{01\cdot0} - p_{00\cdot1} - 2p_{10\cdot1} - 2p_{01\cdot1} - p_{11\cdot1} - p_{02\cdot1}, \\
& p_{00\cdot0} + p_{10\cdot0} + p_{01\cdot0} + p_{11\cdot0} - p_{00\cdot1} - 2p_{10\cdot1} - 2p_{01\cdot1} - 2p_{11\cdot1} - 2p_{02\cdot1}, \\
& p_{00\cdot0} + p_{10\cdot0} + p_{01\cdot0} - p_{00\cdot1} - 2p_{10\cdot1} - 2p_{01\cdot1} - p_{11\cdot1} - 2p_{02\cdot1}, \\
& p_{00\cdot0} - p_{10\cdot0} + p_{01\cdot0} - p_{11\cdot0} - p_{02\cdot0} - p_{00\cdot1} - 2p_{10\cdot1} - 2p_{01\cdot1} - p_{11\cdot1}, \\
& p_{00\cdot0} - p_{10\cdot0} - p_{11\cdot0} - p_{02\cdot0} - p_{00\cdot1} - p_{10\cdot1} - p_{01\cdot1}, \\
& p_{00\cdot0} - p_{10\cdot0} - p_{01\cdot0} - p_{11\cdot0} - p_{02\cdot0} - p_{00\cdot1} - p_{10\cdot1}, \\
& p_{00\cdot0} - p_{00\cdot1} - p_{10\cdot1} - p_{01\cdot1} - p_{11\cdot1} - p_{02\cdot1}, \\
& p_{00\cdot0} + p_{11\cdot0} - p_{00\cdot1} - p_{10\cdot1} - p_{01\cdot1} - 2p_{11\cdot1} - 2p_{02\cdot1}, \\
& p_{00\cdot0} - p_{10\cdot0} - p_{01\cdot0} - p_{00\cdot1} - p_{10\cdot1} - p_{11\cdot1} - p_{02\cdot1}, \\
& p_{00\cdot0} - p_{11\cdot0} - p_{02\cdot0} - p_{00\cdot1} - p_{10\cdot1} - p_{01\cdot1} - p_{02\cdot1}, \\
& p_{00\cdot0} + p_{10\cdot0} - p_{11\cdot0} - p_{02\cdot0} - p_{00\cdot1} - 2p_{10\cdot1} - 2p_{01\cdot1} - 2p_{02\cdot1}, \\
& -p_{10\cdot1} - p_{01\cdot1} - p_{11\cdot1} - p_{02\cdot1}, \\
& -p_{10\cdot0} - p_{01\cdot0} - p_{11\cdot0} - p_{02\cdot0}, \\
& -p_{10\cdot0} - p_{01\cdot0} - 2p_{11\cdot0} - 2p_{02\cdot0} + p_{11\cdot1}, \\
& p_{00\cdot0} + 2p_{11\cdot0} - p_{00\cdot1} - p_{10\cdot1} - 2p_{01\cdot1} - 3p_{11\cdot1} - 3p_{02\cdot1}, \\
& p_{11\cdot0} - p_{10\cdot1} - p_{01\cdot1} - 2p_{11\cdot1} - 2p_{02\cdot1}, \\
& p_{00\cdot0} + p_{10\cdot0} + p_{01\cdot0} + 2p_{11\cdot0} - p_{00\cdot1} - 2p_{10\cdot1} - 2p_{01\cdot1} - 3p_{11\cdot1} - 3p_{02\cdot1}, \\
& -p_{00\cdot0} - 2p_{10\cdot0} - 2p_{01\cdot0} - 2p_{02\cdot0} + p_{00\cdot1} + p_{10\cdot1} - p_{11\cdot1} - p_{02\cdot1}, \\
& -p_{00\cdot0} - p_{10\cdot0} - p_{01\cdot0} - p_{02\cdot0} + p_{00\cdot1} - p_{11\cdot1} - p_{02\cdot1}, \\
& -p_{00\cdot0} - p_{10\cdot0} - p_{01\cdot0} + p_{00\cdot1} - p_{10\cdot1} - p_{11\cdot1} - p_{02\cdot1}, \\
& -p_{00\cdot0} - p_{10\cdot0} + p_{01\cdot0} + p_{00\cdot1} - 2p_{10\cdot1} - 2p_{01\cdot1} - p_{11\cdot1} - p_{02\cdot1}, \\
& -p_{00\cdot0} - p_{10\cdot0} + p_{00\cdot1} - p_{10\cdot1} - p_{01\cdot1} - p_{11\cdot1} - p_{02\cdot1}, \\
& -p_{00\cdot0} - p_{10\cdot0} - 2p_{01\cdot0} - 3p_{11\cdot0} - 3p_{02\cdot0} + p_{00\cdot1} + 2p_{11\cdot1}, \\
& -p_{00\cdot0} - p_{10\cdot0} - p_{01\cdot0} - p_{11\cdot0} - p_{02\cdot0} + p_{00\cdot1}, \\
& -p_{00\cdot0} - p_{10\cdot0} - p_{01\cdot0} - 2p_{11\cdot0} - 2p_{02\cdot0} + p_{00\cdot1} + p_{11\cdot1}, \\
& -p_{00\cdot0} - p_{10\cdot0} - p_{11\cdot0} - p_{02\cdot0} + p_{00\cdot1} - p_{10\cdot1} - p_{01\cdot1}, \\
& -p_{00\cdot0} - p_{10\cdot0} + p_{01\cdot0} - p_{11\cdot0} - p_{02\cdot0} + p_{00\cdot1} - 2p_{10\cdot1} - 2p_{01\cdot1} - p_{11\cdot1}\}
\end{aligned}
$$

and

$$
\begin{aligned}
\phi \leq \min\{&3 - p_{00\cdot 0} - p_{10\cdot 0} - 2p_{01\cdot 0} - p_{11\cdot 0} - p_{00\cdot 1} - 2p_{10\cdot 1} - p_{11\cdot 1} - 3p_{02\cdot 1}, \\
&3 - p_{10\cdot 0} - 2p_{01\cdot 0} - 2p_{00\cdot 1} - 2p_{10\cdot 1} - p_{11\cdot 1} - 3p_{02\cdot 1}, \\
&2 - p_{10\cdot 0} - p_{01\cdot 0} - p_{00\cdot 1} - p_{10\cdot 1} - p_{11\cdot 1} - 2p_{02\cdot 1}, \\
&1 + p_{00\cdot 0} - p_{10\cdot 0} + p_{11\cdot 0} - p_{11\cdot 1} - p_{02\cdot 1}, \\
&1 - p_{10\cdot 0} - p_{02\cdot 1}, \\
&1 + 2p_{00\cdot 0} - p_{10\cdot 0} + p_{01\cdot 0} + 2p_{11\cdot 0} - 2p_{11\cdot 1} - p_{02\cdot 1}, \\
&2 - p_{00\cdot 0} - p_{10\cdot 0} - p_{01\cdot 0} - p_{11\cdot 0} - p_{10\cdot 1} - 2p_{02\cdot 1}, \\
&2 - p_{00\cdot 0} - p_{10\cdot 0} - p_{11\cdot 0} - p_{10\cdot 1} - p_{01\cdot 1} - 2p_{02\cdot 1}, \\
&1 - p_{10\cdot 0} - p_{11\cdot 0} + p_{00\cdot 1} + p_{11\cdot 1} - p_{02\cdot 1}, \\
&1 - 2p_{10\cdot 0} - 2p_{11\cdot 0} - p_{02\cdot 0} + 2p_{00\cdot 1} + p_{10\cdot 1} + p_{01\cdot 1} + 2p_{11\cdot 1}, \\
&1 - p_{11\cdot 0} + p_{00\cdot 1} - p_{10\cdot 1} + p_{11\cdot 1} - p_{02\cdot 1}, \\
&1 - 2p_{11\cdot 0} - p_{02\cdot 0} + 2p_{00\cdot 1} - p_{10\cdot 1} + p_{01\cdot 1} + 2p_{11\cdot 1}, \\
&1 + p_{00\cdot 0} - p_{10\cdot 0} + p_{11\cdot 0} - p_{02\cdot 0} - p_{11\cdot 1}, \\
&1 - p_{10\cdot 0} - p_{02\cdot 0}, \\
&1 - p_{10\cdot 1} - p_{02\cdot 1}, \\
&1 + 2p_{00\cdot 0} + p_{10\cdot 0} + p_{01\cdot 0} + 2p_{11\cdot 0} - 2p_{10\cdot 1} - 2p_{11\cdot 1} - p_{02\cdot 1}, \\
&1 + p_{00\cdot 0} + p_{11\cdot 0} - p_{02\cdot 0} - p_{10\cdot 1} - p_{11\cdot 1}, \\
&2 - p_{00\cdot 0} - p_{10\cdot 0} - p_{11\cdot 0} - 2p_{02\cdot 0} - p_{10\cdot 1} - p_{01\cdot 1}, \\
&1 - p_{11\cdot 0} - p_{02\cdot 0} + p_{00\cdot 1} - p_{10\cdot 1} + p_{11\cdot 1}, \\
&1 - p_{02\cdot 0} - p_{10\cdot 1}, \\
&2 - p_{10\cdot 0} - 2p_{02\cdot 0} - p_{00\cdot 1} - p_{10\cdot 1} - p_{01\cdot 1} - p_{11\cdot 1}, \\
&2 - p_{10\cdot 0} - p_{01\cdot 0} - 2p_{02\cdot 0} - p_{00\cdot 1} - p_{10\cdot 1} - p_{11\cdot 1}, \\
&3 - p_{10\cdot 0} - 2p_{01\cdot 0} - 2p_{02\cdot 0} - 2p_{00\cdot 1} - 2p_{10\cdot 1} - p_{11\cdot 1} - p_{02\cdot 1}, \\
&1 + p_{00\cdot 0} + p_{10\cdot 0} + p_{11\cdot 0} - 2p_{10\cdot 1} - p_{11\cdot 1} - p_{02\cdot 1}, \\
&1 + p_{00\cdot 0} + p_{10\cdot 0} - 2p_{10\cdot 1} - p_{02\cdot 1}, \\
&2 - p_{01\cdot 0} - p_{02\cdot 0} - p_{00\cdot 1} - 2p_{10\cdot 1} - p_{11\cdot 1} - p_{02\cdot 1}, \\
&2 - p_{01\cdot 0} - p_{00\cdot 1} - 2p_{10\cdot 1} - p_{11\cdot 1} - 2p_{02\cdot 1}, \\
&1 + p_{00\cdot 0} + p_{10\cdot 0} - p_{11\cdot 0} + p_{00\cdot 1} - 2p_{10\cdot 1} + p_{11\cdot 1} - p_{02\cdot 1}, \\
&3 - 2p_{00\cdot 0} - 2p_{10\cdot 0} - p_{11\cdot 0} - 3p_{02\cdot 0} - p_{10\cdot 1} - 2p_{01\cdot 1}, \\
&3 - 2p_{00\cdot 0} - 2p_{10\cdot 0} - p_{11\cdot 0} - p_{02\cdot 0} - p_{10\cdot 1} - 2p_{01\cdot 1} - 2p_{02\cdot 1}, \\
&3 - p_{00\cdot 0} - 2p_{10\cdot 0} - p_{11\cdot 0} - 3p_{02\cdot 0} - p_{00\cdot 1} - p_{10\cdot 1} - 2p_{01\cdot 1} - p_{11\cdot 1}, \\
&2 - p_{00\cdot 0} - 2p_{10\cdot 0} - p_{11\cdot 0} - 2p_{02\cdot 0} - p_{01\cdot 1}, \\
&1 - 2p_{10\cdot 0} - p_{02\cdot 0} + p_{00\cdot 1} + p_{10\cdot 1}, \\
&2 - p_{00\cdot 0} - 2p_{10\cdot 0} - p_{11\cdot 0} - p_{02\cdot 0} - p_{01\cdot 1} - p_{02\cdot 1}, \\
&1 + p_{00\cdot 0} - 2p_{10\cdot 0} + p_{11\cdot 0} - p_{02\cdot 0} + p_{00\cdot 1} + p_{10\cdot 1} - p_{11\cdot 1}, \\
&1 - 2p_{10\cdot 0} - p_{11\cdot 0} - p_{02\cdot 0} + p_{00\cdot 1} + p_{10\cdot 1} + p_{11\cdot 1}\}
\end{aligned}
$$

## Noncompliance with no defiers

### Bounds for $\psi$

#### Number of levels of $Y$: 4

$$\psi \geq \max \left\{ \begin{array}{l} 1 - p_{10\cdot 1} - p_{01\cdot 1} - p_{11\cdot 1} - p_{02\cdot 1} - p_{12\cdot 1} - p_{03\cdot 1}, \\ 1 - p_{10\cdot 0} - p_{01\cdot 0} - p_{11\cdot 0} - p_{02\cdot 0} - p_{12\cdot 0} - p_{03\cdot 0}, \\ 1 - p_{11\cdot 0} - p_{02\cdot 0} - p_{12\cdot 0} - p_{03\cdot 0} - p_{10\cdot 1} - p_{01\cdot 1}, \\ 1 - p_{12\cdot 0} - p_{03\cdot 0} - p_{10\cdot 1} - p_{01\cdot 1} - p_{11\cdot 1} - p_{02\cdot 1} \end{array} \right\}$$

$$\psi \leq \min \left\{ \begin{array}{l} 1 + p_{00\cdot 0} + p_{10\cdot 0} + p_{01\cdot 0} + p_{11\cdot 0} + p_{02\cdot 0} + p_{12\cdot 0} - p_{00\cdot 1} - p_{10\cdot 1} - p_{01\cdot 1} - p_{11\cdot 1} - p_{02\cdot 1} - p_{12\cdot 1}, \\ 1, \\ 1 + p_{00\cdot 0} + p_{10\cdot 0} + p_{01\cdot 0} + p_{11\cdot 0} - p_{00\cdot 1} - p_{10\cdot 1} - p_{01\cdot 1} - p_{11\cdot 1}, \\ 1 + p_{00\cdot 0} + p_{10\cdot 0} - p_{00\cdot 1} - p_{10\cdot 1} \end{array} \right\}$$

#### Number of levels of $Y$: 5

$$\psi \geq \max \left\{ \begin{array}{l} 1 - p_{10\cdot 1} - p_{01\cdot 1} - p_{11\cdot 1} - p_{02\cdot 1} - p_{12\cdot 1} - p_{03\cdot 1} - p_{13\cdot 1} - p_{04\cdot 1}, \\ 1 - p_{13\cdot 0} - p_{04\cdot 0} - p_{10\cdot 1} - p_{01\cdot 1} - p_{11\cdot 1} - p_{02\cdot 1} - p_{12\cdot 1} - p_{03\cdot 1}, \\ 1 - p_{10\cdot 0} - p_{01\cdot 0} - p_{11\cdot 0} - p_{02\cdot 0} - p_{12\cdot 0} - p_{03\cdot 0} - p_{13\cdot 0} - p_{04\cdot 0}, \\ 1 - p_{11\cdot 0} - p_{02\cdot 0} - p_{12\cdot 0} - p_{03\cdot 0} - p_{13\cdot 0} - p_{04\cdot 0} - p_{10\cdot 1} - p_{01\cdot 1}, \\ 1 - p_{12\cdot 0} - p_{03\cdot 0} - p_{13\cdot 0} - p_{04\cdot 0} - p_{10\cdot 1} - p_{01\cdot 1} - p_{11\cdot 1} - p_{02\cdot 1} \end{array} \right\}$$

$$\psi \leq \min \left\{ \begin{array}{l} 1 + p_{00\cdot 0} + p_{10\cdot 0} - p_{00\cdot 1} - p_{10\cdot 1}, \\ 1 + p_{00\cdot 0} + p_{10\cdot 0} + p_{01\cdot 0} + p_{11\cdot 0} + p_{02\cdot 0} + p_{12\cdot 0} + p_{03\cdot 0} + p_{13\cdot 0} - p_{00\cdot 1} - p_{10\cdot 1} - p_{01\cdot 1} - p_{11\cdot 1} - \\ \quad p_{02\cdot 1} - p_{12\cdot 1} - p_{03\cdot 1} - p_{13\cdot 1}, \\ 1, \\ 1 + p_{00\cdot 0} + p_{10\cdot 0} + p_{01\cdot 0} + p_{11\cdot 0} + p_{02\cdot 0} + p_{12\cdot 0} - p_{00\cdot 1} - p_{10\cdot 1} - p_{01\cdot 1} - p_{11\cdot 1} - p_{02\cdot 1} - p_{12\cdot 1}, \\ 1 + p_{00\cdot 0} + p_{10\cdot 0} + p_{01\cdot 0} + p_{11\cdot 0} - p_{00\cdot 1} - p_{10\cdot 1} - p_{01\cdot 1} - p_{11\cdot 1} \end{array} \right\}$$

## Bounds for $\theta$

### Number of levels of $Y$: 4

$$\theta \geq \max \begin{cases} p_{00\cdot 0} + p_{10\cdot 0} + p_{01\cdot 0} + p_{11\cdot 0} - p_{00\cdot 1} - p_{10\cdot 1} - p_{01\cdot 1} - p_{11\cdot 1}, \\ p_{00\cdot 0} + p_{10\cdot 0} - p_{00\cdot 1} - p_{10\cdot 1}, \\ 0, \\ p_{00\cdot 0} + p_{10\cdot 0} + p_{01\cdot 0} + p_{11\cdot 0} + p_{02\cdot 0} + p_{12\cdot 0} - p_{00\cdot 1} - p_{10\cdot 1} - p_{01\cdot 1} - p_{11\cdot 1} - p_{02\cdot 1} - p_{12\cdot 1} \end{cases}$$

$$\theta \leq \min \begin{cases} 1 + p_{00\cdot 0} + p_{11\cdot 0} - p_{00\cdot 1} - p_{10\cdot 1} - p_{11\cdot 1} - p_{03\cdot 1}, \\ 1 - p_{10\cdot 0} - p_{03\cdot 0}, \\ 1 + p_{00\cdot 0} + p_{01\cdot 0} + p_{11\cdot 0} + p_{12\cdot 0} - p_{00\cdot 1} - p_{10\cdot 1} - p_{01\cdot 1} - p_{11\cdot 1} - p_{12\cdot 1} - p_{03\cdot 1}, \\ 1 - p_{10\cdot 1} - p_{03\cdot 1} \end{cases}$$

### Number of levels of $Y$: 5

$$\theta \geq \max \begin{cases} p_{00\cdot 0} + p_{10\cdot 0} + p_{01\cdot 0} + p_{11\cdot 0} - p_{00\cdot 1} - p_{10\cdot 1} - p_{01\cdot 1} - p_{11\cdot 1}, \\ p_{00\cdot 0} + p_{10\cdot 0} - p_{00\cdot 1} - p_{10\cdot 1}, \\ 0, \\ p_{00\cdot 0} + p_{10\cdot 0} + p_{01\cdot 0} + p_{11\cdot 0} + p_{02\cdot 0} + p_{12\cdot 0} - p_{00\cdot 1} - p_{10\cdot 1} - p_{01\cdot 1} - p_{11\cdot 1} - p_{02\cdot 1} - p_{12\cdot 1}, \\ p_{00\cdot 0} + p_{10\cdot 0} + p_{01\cdot 0} + p_{11\cdot 0} + p_{02\cdot 0} + p_{12\cdot 0} + p_{03\cdot 0} + p_{13\cdot 0} - p_{00\cdot 1} - p_{10\cdot 1} - p_{01\cdot 1} - p_{11\cdot 1} - \\ \quad p_{02\cdot 1} - p_{12\cdot 1} - p_{03\cdot 1} - p_{13\cdot 1} \end{cases}$$

$$\theta \leq \min \begin{cases} 1 + p_{00\cdot 0} + p_{11\cdot 0} - p_{00\cdot 1} - p_{10\cdot 1} - p_{11\cdot 1} - p_{04\cdot 1}, \\ 1 + p_{00\cdot 0} + p_{01\cdot 0} + p_{11\cdot 0} + p_{12\cdot 0} - p_{00\cdot 1} - p_{10\cdot 1} - p_{01\cdot 1} - p_{11\cdot 1} - p_{12\cdot 1} - p_{04\cdot 1}, \\ 1 - p_{10\cdot 0} - p_{04\cdot 0}, \\ 1 + p_{00\cdot 0} + p_{01\cdot 0} + p_{11\cdot 0} + p_{02\cdot 0} + p_{12\cdot 0} + p_{13\cdot 0} - p_{00\cdot 1} - p_{10\cdot 1} - p_{01\cdot 1} - p_{11\cdot 1} - p_{02\cdot 1} - \\ \quad p_{12\cdot 1} - p_{13\cdot 1} - p_{04\cdot 1}, \\ 1 - p_{10\cdot 1} - p_{04\cdot 1} \end{cases}$$

### Bounds for $\phi$

### Number of levels of $Y$: 4

$$\phi \geq \max \begin{cases} p_{00\cdot 0} + p_{10\cdot 0} + p_{01\cdot 0} - p_{12\cdot 0} - p_{03\cdot 0} - p_{00\cdot 1} - 2p_{10\cdot 1} - 2p_{01\cdot 1} - p_{11\cdot 1} - p_{02\cdot 1}, \\ p_{00\cdot 0} + p_{10\cdot 0} + p_{01\cdot 0} - p_{00\cdot 1} - 2p_{10\cdot 1} - 2p_{01\cdot 1} - p_{11\cdot 1} - p_{02\cdot 1} - p_{12\cdot 1} - p_{03\cdot 1}, \\ p_{00\cdot 0} - p_{00\cdot 1} - p_{10\cdot 1} - p_{01\cdot 1} - p_{11\cdot 1} - p_{02\cdot 1} - p_{12\cdot 1} - p_{03\cdot 1}, \\ p_{00\cdot 0} - p_{11\cdot 0} - p_{02\cdot 0} - p_{12\cdot 0} - p_{03\cdot 0} - p_{00\cdot 1} - p_{10\cdot 1} - p_{01\cdot 1}, \\ p_{00\cdot 0} - p_{12\cdot 0} - p_{03\cdot 0} - p_{00\cdot 1} - p_{10\cdot 1} - p_{01\cdot 1} - p_{11\cdot 1} - p_{02\cdot 1}, \\ p_{00\cdot 0} + p_{10\cdot 0} + p_{01\cdot 0} + p_{11\cdot 0} + p_{02\cdot 0} - p_{00\cdot 1} - 2p_{10\cdot 1} - 2p_{01\cdot 1} - 2p_{11\cdot 1} - 2p_{02\cdot 1} - p_{12\cdot 1} - p_{03\cdot 1} \end{cases}$$

$$\phi \leq \min \begin{cases} 1 - p_{03\cdot 0} - p_{10\cdot 1}, \\ 1 + p_{00\cdot 0} + p_{01\cdot 0} + p_{11\cdot 0} + p_{12\cdot 0} - p_{03\cdot 0} - p_{00\cdot 1} - p_{10\cdot 1} - p_{01\cdot 1} - p_{11\cdot 1} - p_{12\cdot 1}, \\ 1 + p_{00\cdot 0} + p_{11\cdot 0} - p_{03\cdot 0} - p_{00\cdot 1} - p_{10\cdot 1} - p_{11\cdot 1}, \\ 1 + p_{00\cdot 0} + p_{10\cdot 0} + p_{01\cdot 0} + p_{11\cdot 0} + p_{12\cdot 0} - p_{00\cdot 1} - 2p_{10\cdot 1} - p_{01\cdot 1} - p_{11\cdot 1} - p_{12\cdot 1} - p_{03\cdot 1}, \\ 1 + 2p_{00\cdot 0} + p_{10\cdot 0} + p_{01\cdot 0} + 2p_{11\cdot 0} + p_{12\cdot 0} - 2p_{00\cdot 1} - 2p_{10\cdot 1} - p_{01\cdot 1} - 2p_{11\cdot 1} - p_{12\cdot 1} - p_{03\cdot 1}, \\ 1 + p_{00\cdot 0} + p_{10\cdot 0} + p_{11\cdot 0} - p_{00\cdot 1} - 2p_{10\cdot 1} - p_{11\cdot 1} - p_{03\cdot 1} \end{cases}$$

### Number of levels of $Y$: 5

$$\phi \geq \max \begin{cases} p_{00\cdot 0} + p_{10\cdot 0} + p_{01\cdot 0} - p_{12\cdot 0} - p_{03\cdot 0} - p_{13\cdot 0} - p_{04\cdot 0} - p_{00\cdot 1} - 2p_{10\cdot 1} - 2p_{01\cdot 1} - p_{11\cdot 1} - p_{02\cdot 1}, \\ p_{00\cdot 0} + p_{10\cdot 0} + p_{01\cdot 0} - p_{13\cdot 0} - p_{04\cdot 0} - p_{00\cdot 1} - 2p_{10\cdot 1} - 2p_{01\cdot 1} - p_{11\cdot 1} - p_{02\cdot 1} - p_{12\cdot 1} - p_{03\cdot 1}, \\ p_{00\cdot 0} + p_{10\cdot 0} + p_{01\cdot 0} - p_{00\cdot 1} - 2p_{10\cdot 1} - 2p_{01\cdot 1} - p_{11\cdot 1} - p_{02\cdot 1} - p_{12\cdot 1} - p_{03\cdot 1} - p_{13\cdot 1} - p_{04\cdot 1}, \\ p_{00\cdot 0} - p_{00\cdot 1} - p_{10\cdot 1} - p_{01\cdot 1} - p_{11\cdot 1} - p_{02\cdot 1} - p_{12\cdot 1} - p_{03\cdot 1} - p_{13\cdot 1} - p_{04\cdot 1}, \\ p_{00\cdot 0} - p_{11\cdot 0} - p_{02\cdot 0} - p_{12\cdot 0} - p_{03\cdot 0} - p_{13\cdot 0} - p_{04\cdot 0} - p_{00\cdot 1} - p_{10\cdot 1} - p_{01\cdot 1}, \\ p_{00\cdot 0} - p_{12\cdot 0} - p_{03\cdot 0} - p_{13\cdot 0} - p_{04\cdot 0} - p_{00\cdot 1} - p_{10\cdot 1} - p_{01\cdot 1} - p_{11\cdot 1} - p_{02\cdot 1}, \\ p_{00\cdot 0} - p_{13\cdot 0} - p_{04\cdot 0} - p_{00\cdot 1} - p_{10\cdot 1} - p_{01\cdot 1} - p_{11\cdot 1} - p_{02\cdot 1} - p_{12\cdot 1} - p_{03\cdot 1}, \\ p_{00\cdot 0} + p_{10\cdot 0} + p_{01\cdot 0} + p_{11\cdot 0} + p_{02\cdot 0} - p_{00\cdot 1} - 2p_{10\cdot 1} - 2p_{01\cdot 1} - 2p_{11\cdot 1} - 2p_{02\cdot 1} - p_{12\cdot 1} - \\ \quad p_{03\cdot 1} - p_{13\cdot 1} - p_{04\cdot 1}, \\ p_{00\cdot 0} + p_{10\cdot 0} + p_{01\cdot 0} + p_{11\cdot 0} + p_{02\cdot 0} - p_{13\cdot 0} - p_{04\cdot 0} - p_{00\cdot 1} - 2p_{10\cdot 1} - 2p_{01\cdot 1} - 2p_{11\cdot 1} - \\ \quad 2p_{02\cdot 1} - p_{12\cdot 1} - p_{03\cdot 1}, \\ p_{00\cdot 0} + p_{10\cdot 0} + p_{01\cdot 0} + p_{11\cdot 0} + p_{02\cdot 0} + p_{12\cdot 0} + p_{03\cdot 0} - p_{00\cdot 1} - 2p_{10\cdot 1} - 2p_{01\cdot 1} - 2p_{11\cdot 1} - \\ \quad 2p_{02\cdot 1} - 2p_{12\cdot 1} - 2p_{03\cdot 1} - p_{13\cdot 1} - p_{04\cdot 1} \end{cases}$$

$$
\phi \leq \min \left\{ \begin{array}{l}
1 + 2p_{00\cdot 0} + p_{10\cdot 0} + p_{01\cdot 0} + 2p_{11\cdot 0} + p_{12\cdot 0} - 2p_{00\cdot 1} - 2p_{10\cdot 1} - p_{01\cdot 1} - 2p_{11\cdot 1} - p_{12\cdot 1} - p_{04\cdot 1}, \\
1 + p_{00\cdot 0} + p_{10\cdot 0} + p_{01\cdot 0} + p_{11\cdot 0} + p_{12\cdot 0} - p_{00\cdot 1} - 2p_{10\cdot 1} - p_{01\cdot 1} - p_{11\cdot 1} - p_{12\cdot 1} - p_{04\cdot 1}, \\
1 + 2p_{00\cdot 0} + p_{10\cdot 0} + 2p_{01\cdot 0} + 2p_{11\cdot 0} + p_{02\cdot 0} + 2p_{12\cdot 0} + p_{13\cdot 0} - 2p_{00\cdot 1} - 2p_{10\cdot 1} - 2p_{01\cdot 1} - \\
2p_{11\cdot 1} - p_{02\cdot 1} - 2p_{12\cdot 1} - p_{13\cdot 1} - p_{04\cdot 1}, \\
1 + 2p_{00\cdot 0} + p_{10\cdot 0} + p_{01\cdot 0} + 2p_{11\cdot 0} + p_{02\cdot 0} + p_{12\cdot 0} + p_{13\cdot 0} - 2p_{00\cdot 1} - 2p_{10\cdot 1} - p_{01\cdot 1} - \\
2p_{11\cdot 1} - p_{02\cdot 1} - p_{12\cdot 1} - p_{13\cdot 1} - p_{04\cdot 1}, \\
1 + p_{00\cdot 0} + p_{10\cdot 0} + p_{01\cdot 0} + p_{11\cdot 0} + p_{02\cdot 0} + p_{12\cdot 0} + p_{13\cdot 0} - p_{00\cdot 1} - 2p_{10\cdot 1} - p_{01\cdot 1} - p_{11\cdot 1} - \\
p_{02\cdot 1} - p_{12\cdot 1} - p_{13\cdot 1} - p_{04\cdot 1}, \\
1 + p_{00\cdot 0} + p_{11\cdot 0} - p_{04\cdot 0} - p_{00\cdot 1} - p_{10\cdot 1} - p_{11\cdot 1}, \\
1 + p_{00\cdot 0} + p_{01\cdot 0} + p_{11\cdot 0} + p_{12\cdot 0} - p_{04\cdot 0} - p_{00\cdot 1} - p_{10\cdot 1} - p_{01\cdot 1} - p_{11\cdot 1} - p_{12\cdot 1}, \\
1 + p_{00\cdot 0} + p_{01\cdot 0} + p_{11\cdot 0} + p_{02\cdot 0} + p_{12\cdot 0} + p_{13\cdot 0} - p_{04\cdot 0} - p_{00\cdot 1} - p_{10\cdot 1} - p_{01\cdot 1} - p_{11\cdot 1} - \\
p_{02\cdot 1} - p_{12\cdot 1} - p_{13\cdot 1}, \\
1 - p_{04\cdot 0} - p_{10\cdot 1}, \\
1 + p_{00\cdot 0} + p_{10\cdot 0} + p_{11\cdot 0} - p_{00\cdot 1} - 2p_{10\cdot 1} - p_{11\cdot 1} - p_{04\cdot 1}
\end{array} \right\}
$$

## References


Michael C Sachs, Gustav Jonzon, Arvid Sjölander, and Erin E Gabriel. A general method for deriving tight symbolic bounds on causal effects. *Journal of Computational and Graphical Statistics*, (just-accepted):1–23, 2022.
